# Supplementary material for: Error Control and Automatic Detection of Reference Active Spaces in Many-Body Expanded Full Configuration Interaction
Source: arXiv:2406.11343 ancillary file (2024-06-17)
Supplement: Supplementary file 1 [file si.pdf]

# Supporting Information: Error Control and Automatic Detection of Reference Active Spaces in Many-Body Expanded Full Configuration Interaction

Jonas Greiner,† Jürgen Gauss,*,† and Janus J. Eriksen*,‡

†*Department Chemie, Johannes Gutenberg-Universität Mainz*

*Duesbergweg 10–14, 55128 Mainz, Germany*

‡*DTU Chemistry, Technical University of Denmark*

*Kemitorvet Bldg. 206, 2800 Kgs. Lyngby, Denmark*

E-mail: gauss@uni-mainz.de; janus@dtu.dk

# 1 Reference Space Detection

For every orbital tuple, the state which produces the maximum quantum fidelity with the reference space wave function is used to construct the respective increment. This state is determined iteratively for every individual increment using the algorithm in Fig. S1.

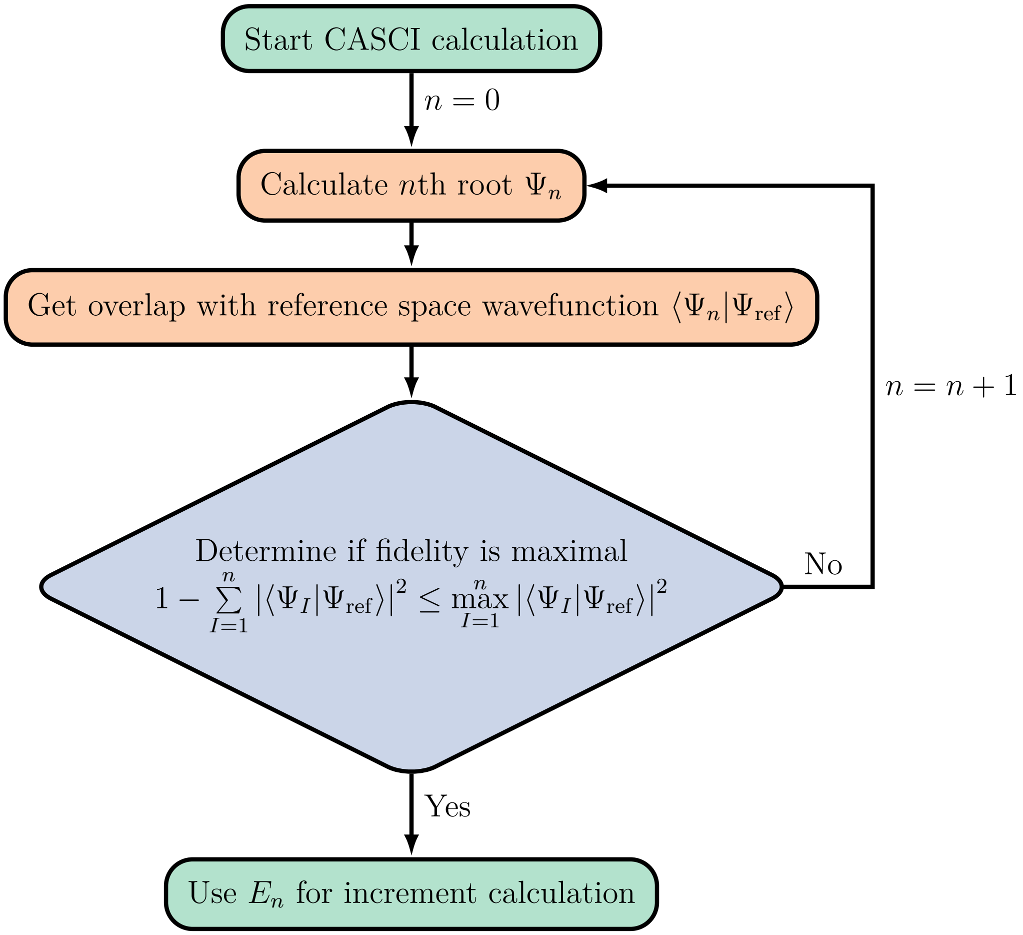


Figure S1: Flowchart for the root-finding algorithm.

The Davidson procedure is started with the reference space wave function as initial guess and restarted using the roots from the previous iteration. The decision step in Fig. S1 will ensure that the state with the maximum quantum fidelity is determined in as few iterations as possible. The algorithm will attempt to target only a desired spin state by providing a suitable initial guess or through level-shifting of undesirable spin states.[S1] Whenever states

of different spins are eigenfunctions corresponding to a specific spin projection quantum number, the decision step in Fig. S1 might not trigger before all states of a given spin have been considered. However, when the ground state is targeted, the algorithm rarely moves beyond the first root. We have also experimented with directly targeting the desired state through root-homing, which is often inefficient due to convergence issues.[S2]

Following every MBE order, the tuple that produces the lowest quantum fidelity $\min_I F_{I,\text{ref}}$ alongside all tuples with fidelities within 1% of $1 - \min_I F_{I,\text{ref}}$ are considered. From the union of all MOs in these tuples, the orbitals with the highest occurrence are added to the reference space. If the highest occurrence is one, either because only one tuple of orbitals is considered or because there is no intersection between the considered tuples, all orbitals are added. This procedure ensures that the orbitals that are most likely to be responsible for any changes to the wave function are added to the reference space. The dynamic fidelity threshold is defined by the sigmoid function in Fig. S2 such that reference spaces will never grow beyond impractical dimensions.

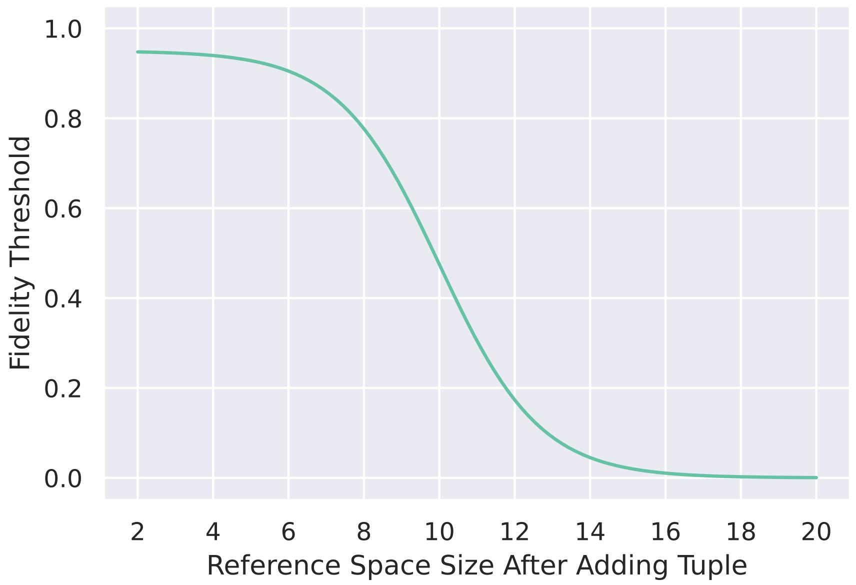


Figure S2: Sigmoid function used as quantum fidelity threshold. Starting threshold is 0.95.

# 2 Orbital Clustering

The orbital clustering algorithm requires a desired cluster size, $n_{\max}$, and a maximum MBE order, $k$, as input arguments, the latter which describes up to what order in an MBE information is to be gathered for identifying clusters. First, clusters that are as homogeneous as possible in both size and occupation are predetermined from the total number of electrons and orbitals in the expansion space. A single-orbital MBE is then performed through order $k$, and increment magnitudes for all tuples that include a given orbital pair are accumulated.

This procedure gives rise to a symmetric contribution matrix with a vanishing diagonal. In order to maximize both intra-cluster and early-order contributions, pair contributions within blocks formed on the basis of predetermined cluster sizes and occupations must be maximized. The resulting optimization problem is of combinatorial nature and exhibits many local maxima. While it is not necessary to locate a global maximum, the evaluation of the score function is comparatively cheap, and we have thus opted for simulated annealing with a slow exponential cooling schedule to maximize these contributions. The starting temperature, $T_{\text{start}}$, is determined automatically by employing the method suggested by Ben-Ameur and enforcing an acceptance rate of 0.99 for 1000 random samples, each with one random neighbor that reduces the cost function.[S3] Annealing is done until the score function does not increase for a set number of iterations, usually around 100,000, and the temperature scheduling parameter, $\alpha$, is set such that it decreases to $10^{-5}$ over the iterative loop. A summary of this orbital clustering algorithm is provided in Fig. S3.

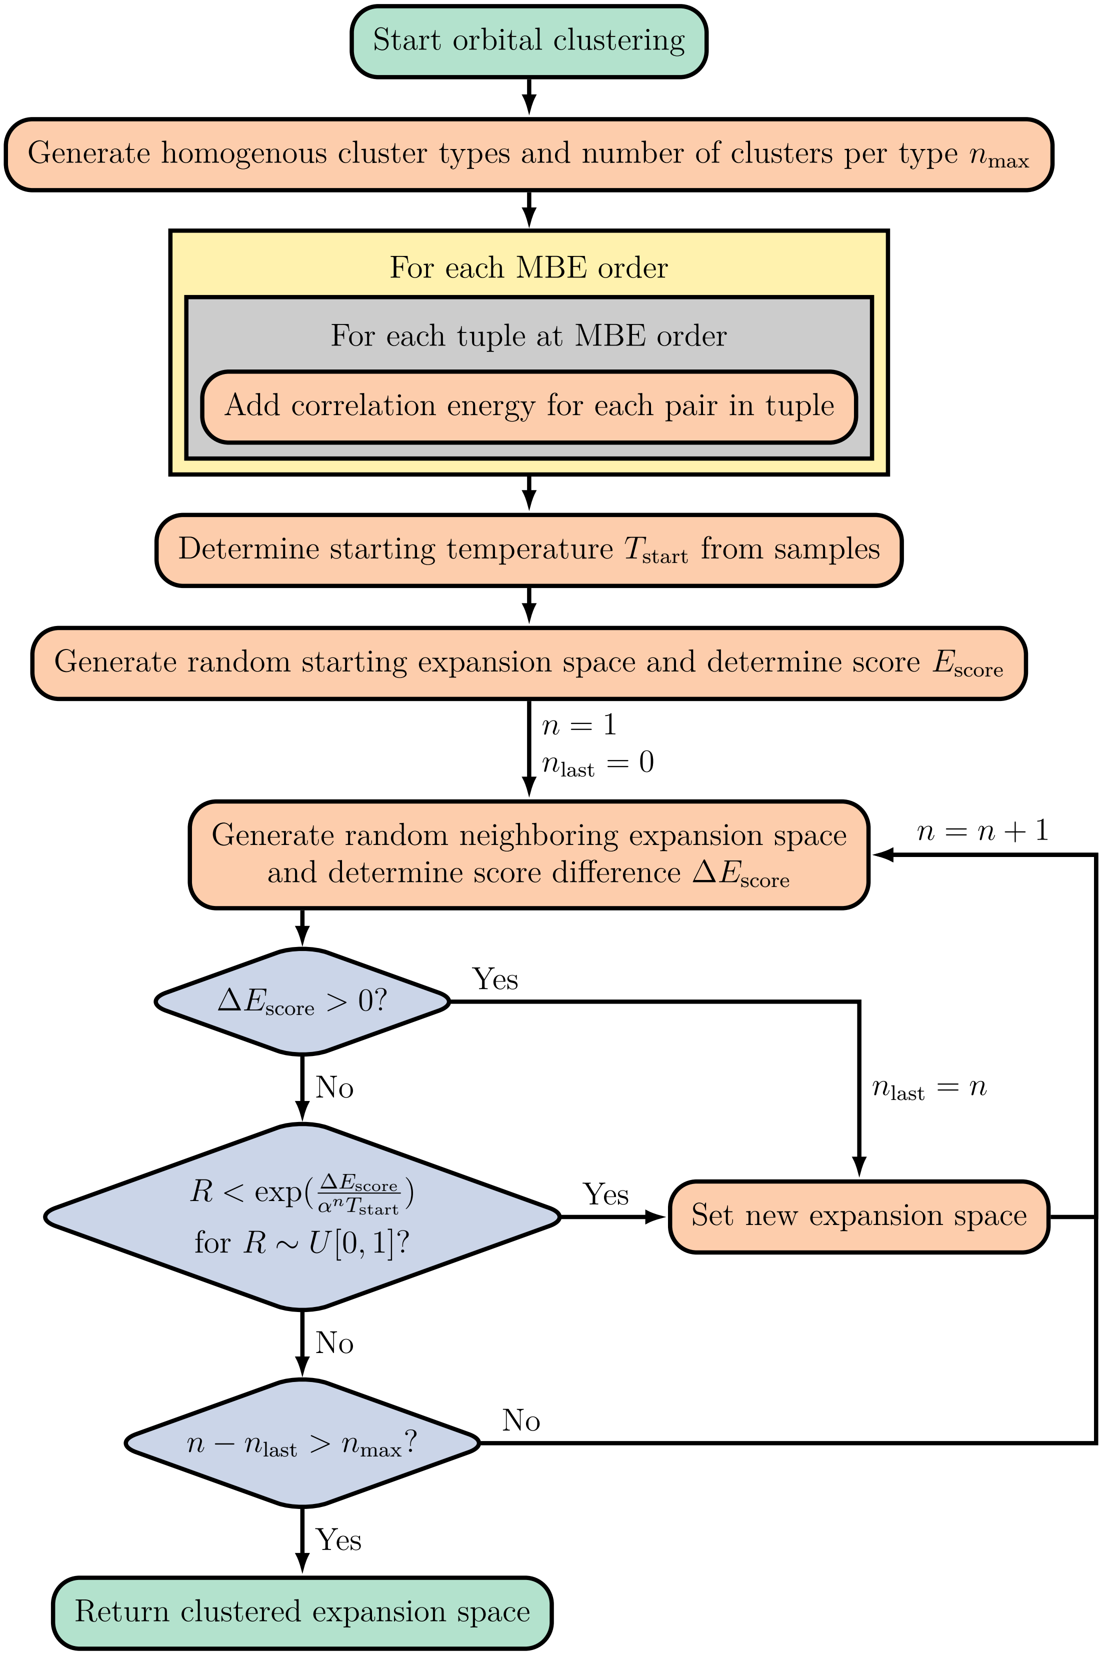


Figure S3: Flowchart for the orbital clustering algorithm.

# 3 Error Control and Orbital Screening

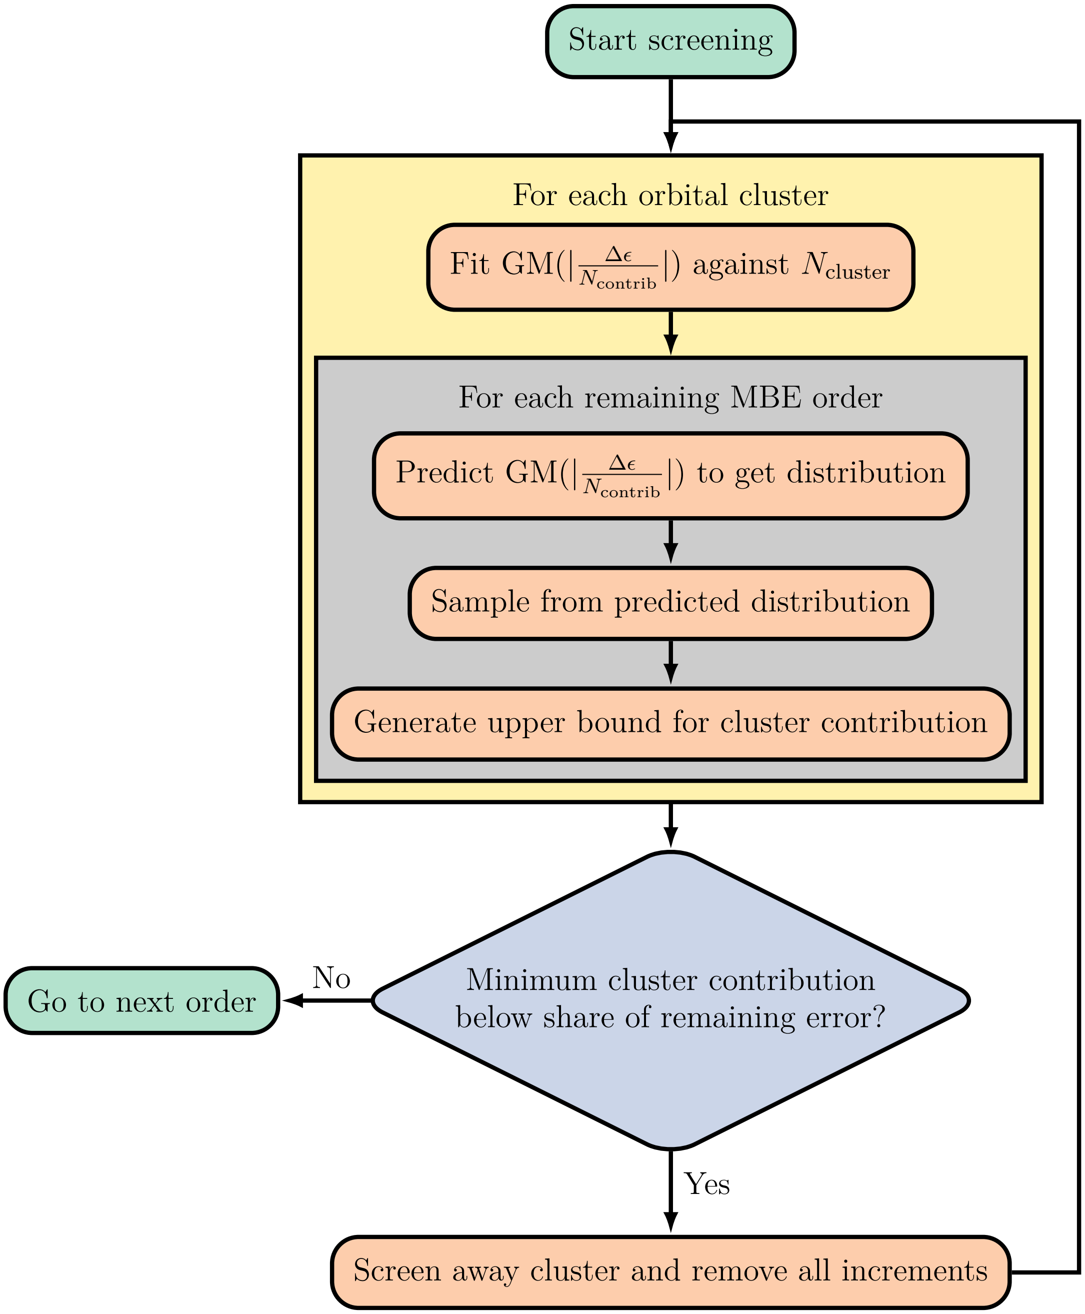


Figure S4: Flowchart for the screening and error estimation procedure.

An illustration of our new screening protocol is provided in Fig. S4. Here, cluster-based screening is controlled by estimating the errors accrued at future orders if some cluster is removed from the expansion space at the current order. The error estimation is accom-

plished in two steps: fitting and sampling. The sampling step requires a limited number of increments at current and previous orders, which are obtained by randomly choosing a maximum of 10,000 increments from the last $\max_i(n(S_i))$ orders with replacement. This number describes the maximum cardinality of the orbital clusters, $S_i$, thus ensuring that the sample includes increments from all clusters. The probability density for this sample is then estimated through kernel density estimation[S4,S5] (KDE). After a sample of increments and the corresponding probabilities have been prepared, fitting is started by looping over all possible clusters at remaining orders.

For a given error threshold, $\Delta E_{\text{thres}}$, orbitals are only considered for screening if at least 3 data points are present and all $x + 1$ orbital contributions (where $x$ is the exponent of $\Delta E_{\text{thres}}$ in scientific notation) have been calculated. This restriction is necessary to ensure that enough data is present to enable confident error predictions. After reaching this point in the expansion, a weighted linear least-squares fit of the geometric mean of the normalized increment magnitudes, $\text{GM}(|\frac{\Delta\epsilon}{N_{\text{contrib}}}|)$, against the number of clusters in the orbital tuples is carried out on the logarithmic scale for the individual orbital clusters. The weights are calculated as the inverse of the variance of the geometric sample mean on the logarithmic scale. The upper prediction interval for a given confidence level is then used to make predictions of $\text{GM}(|\frac{\Delta\epsilon}{N_{\text{contrib}}}|)$ at later orders in the expansion.

The linear relationship of $\log\left(\text{GM}(|\frac{\Delta\epsilon}{N_{\text{contrib}}}|)\right)$ with respect to the number of clusters will deteriorate upon an increase in the CASCI convergence criterion, as can be seen in Fig. S5. The deviation from linearity at tighter convergence criteria is mostly caused by the numerical limits of double-precision arithmetics. We have found this behavior not to be problematic unless very high accuracy is required, given how the affected increments are small in magnitude and have arbitrary signs that will cancel out. The variance of the log-transformed normalized increment magnitudes for the last data point is used to calculate the prediction

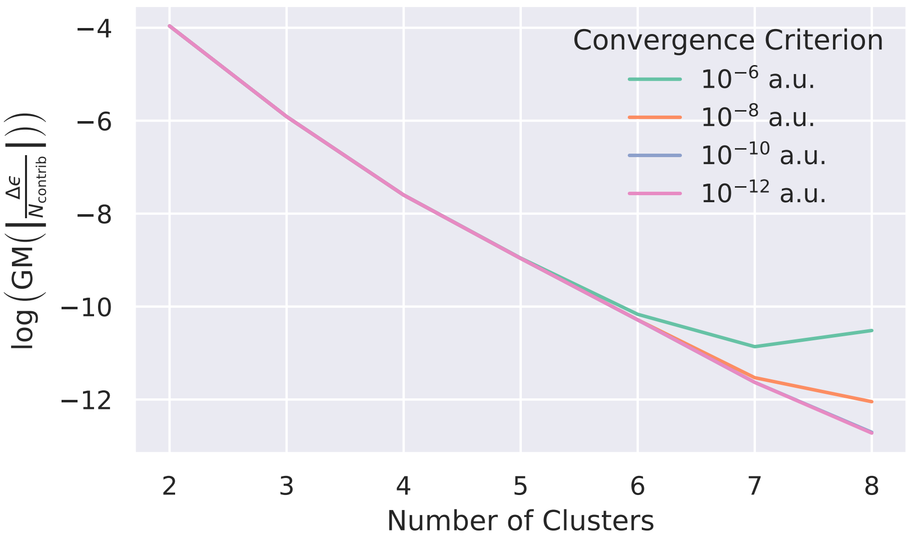


Figure S5: Log-transformed geometric mean of the normalized increment magnitude plotted against number of clusters for various CASCI convergence thresholds at expansion orders ($k \leq 8$) for a single-orbital MBE-FCI calculation of $H_2O$/cc-pVTZ based on an empty reference space. Orbital clusters comprising between 1-4 MOs have been selected at random.

interval and also to construct the normal distributions that are required to sample increment contributions in the sampling. This treatment of the variance yields a good approximation as the variance of the logarithm generally stays constant upon reaching a certain sample size.

The confidence level, $\gamma$, used to calculate the prediction interval is chosen such that it decreases depending on the state of convergence. It starts at 95% and then decreases to 80% whenever the cumulative sum of the increment contributions over the last $\max_i(n(S_i))$ orders is smaller than the remaining possible error. It then further decreases to 50% and then 5% when the cumulative sum of the increment contributions stays below the remaining possible error for two or three times $\max_i(n(S_i))$ orders, respectively. This approach effectively encodes the assumption that less confidence in the error estimation is needed when the current MBE orders already produce contributions below the error bound. Simultaneously, this treatment also ensures that errors are not grossly overestimated due to large prediction intervals, and that the MBE can be properly terminated when convergence is reached.

After $\mathrm{GM}(|\frac{\Delta\epsilon}{N_{\mathrm{contrib}}}|)$ has been predicted for a given orbital cluster and order, the increments for current and previous orders are sampled according to the predicted normal distribution using importance sampling. Increments are sampled based on the logarithm of their magnitude, while the sum of these increments is constructed from their actual value. A maximum of 1,000 increment samples are taken at a time, a procedure which is executed for all distributions necessary to describe the increments spawning from a given cluster at a given MBE order. The sampling is continued until the $\gamma$th quantile of the increment sum is converged, and this is used as an upper bound for the contribution of this cluster at the predicted order. The proposed procedure is repeated for the remaining orders until the last $\max_i(n(S_i))$ orders have not contributed to more than 1% of the total accumulated error for this cluster. Possible sign cancellation between the contributions at different orders is not considered.

After potential contributions for all orbital clusters have been estimated, the orbital cluster with the smallest contribution is screened away if it contributes less than its allotted share of the remaining error threshold. This share is calculated by multiplying the remaining error by the ratio of the cluster's increments and the total number of increments for the next $\max_i(n(S_i))$ orders. When a cluster is screened away, all increments spawning from this cluster are removed from $\mathrm{GM}(|\frac{\Delta\epsilon}{N_{\mathrm{contrib}}}|)$, and the procedure is repeated until all orbital clusters contribute more than their allotted share, after which the MBE resumes, or until no further increments can be constructed from the remaining expansion space.

# 4 Additional Results for Ammonia and Methane

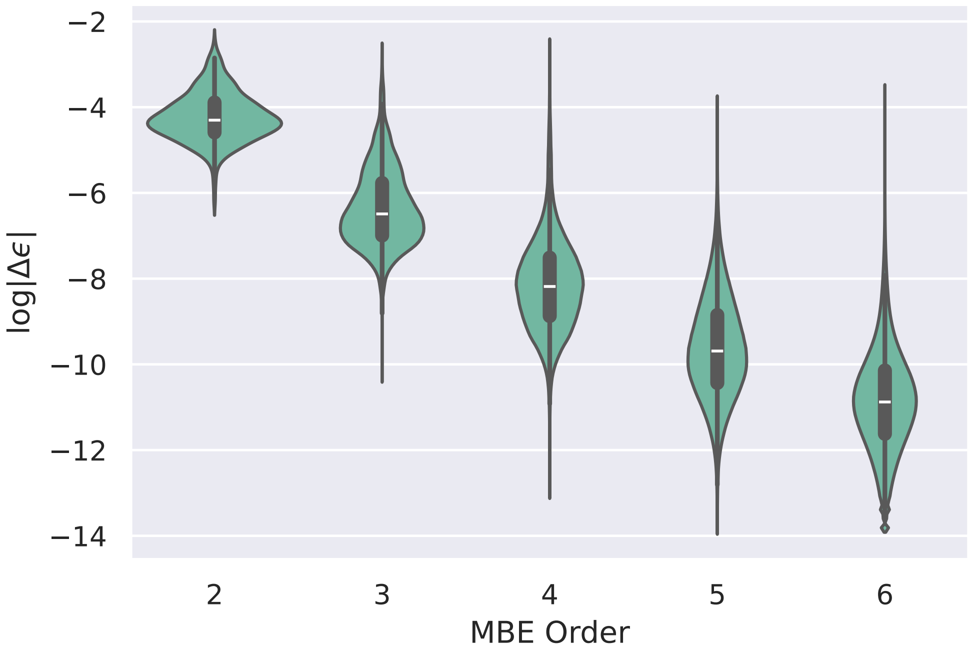


Figure S6: Results for $NH_3$/cc-pVTZ on par with Fig. 1 of the main study.

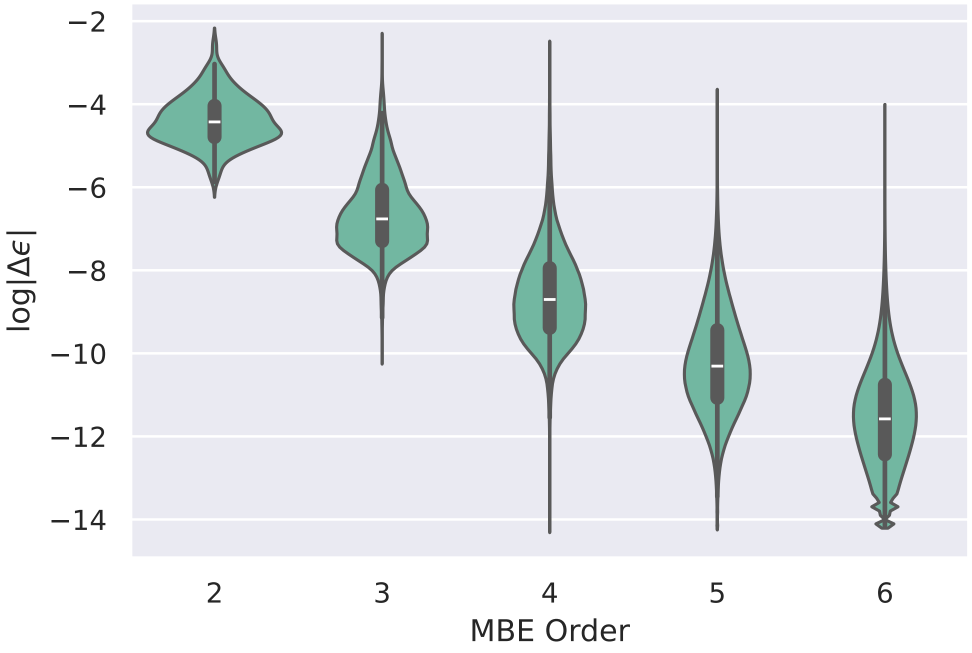


Figure S7: Results for $CH_4$/cc-pVTZ on par with Fig. 1 of the main study.

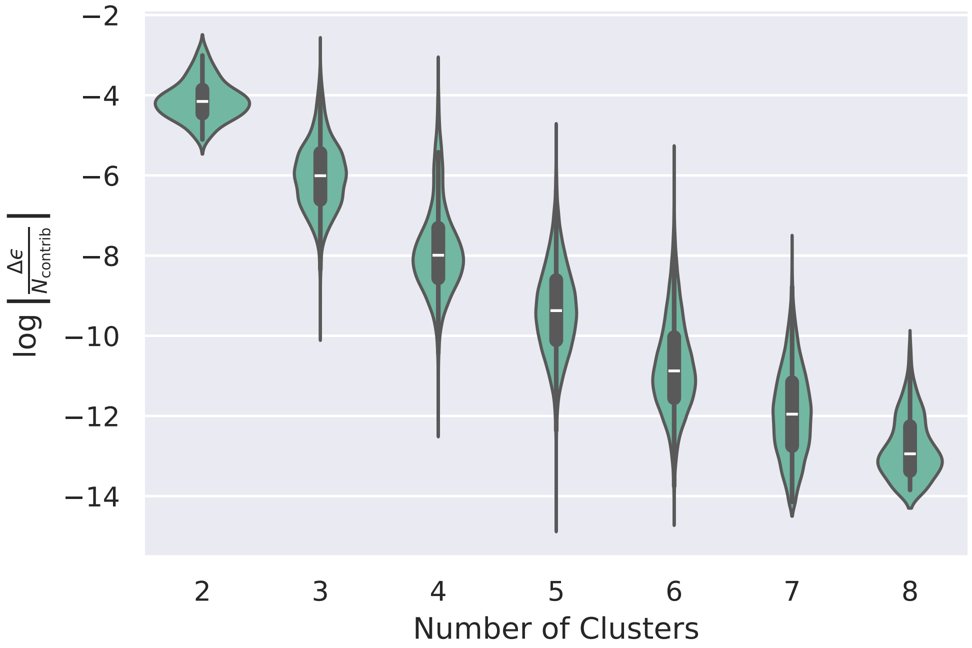


Figure S8: Results for $NH_3$/cc-pVTZ on par with Fig. 2 of the main study.

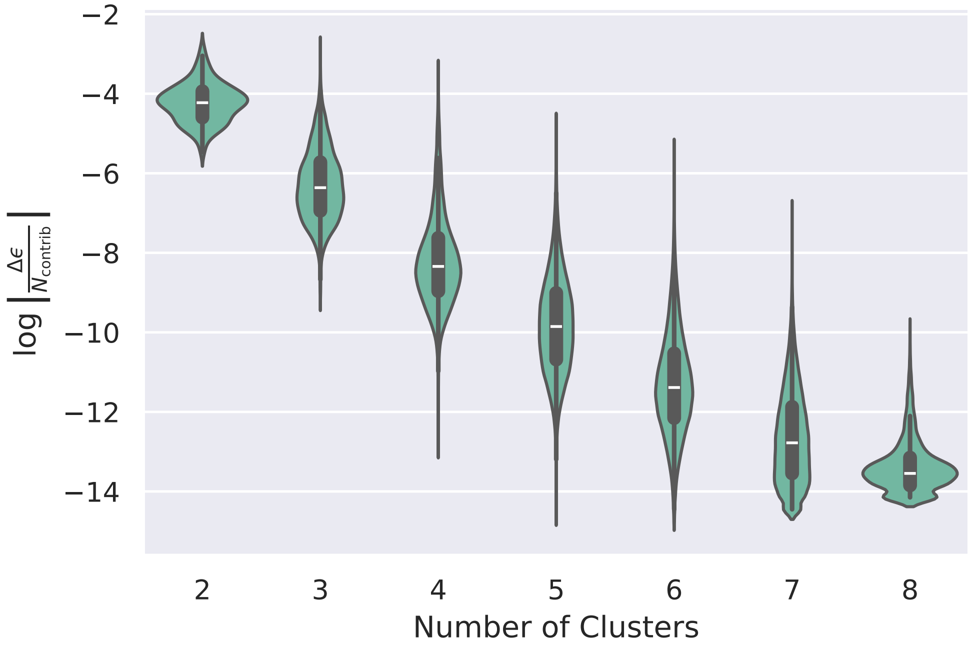


Figure S9: Results for $CH_4$/cc-pVTZ on par with Fig. 2 of the main study.

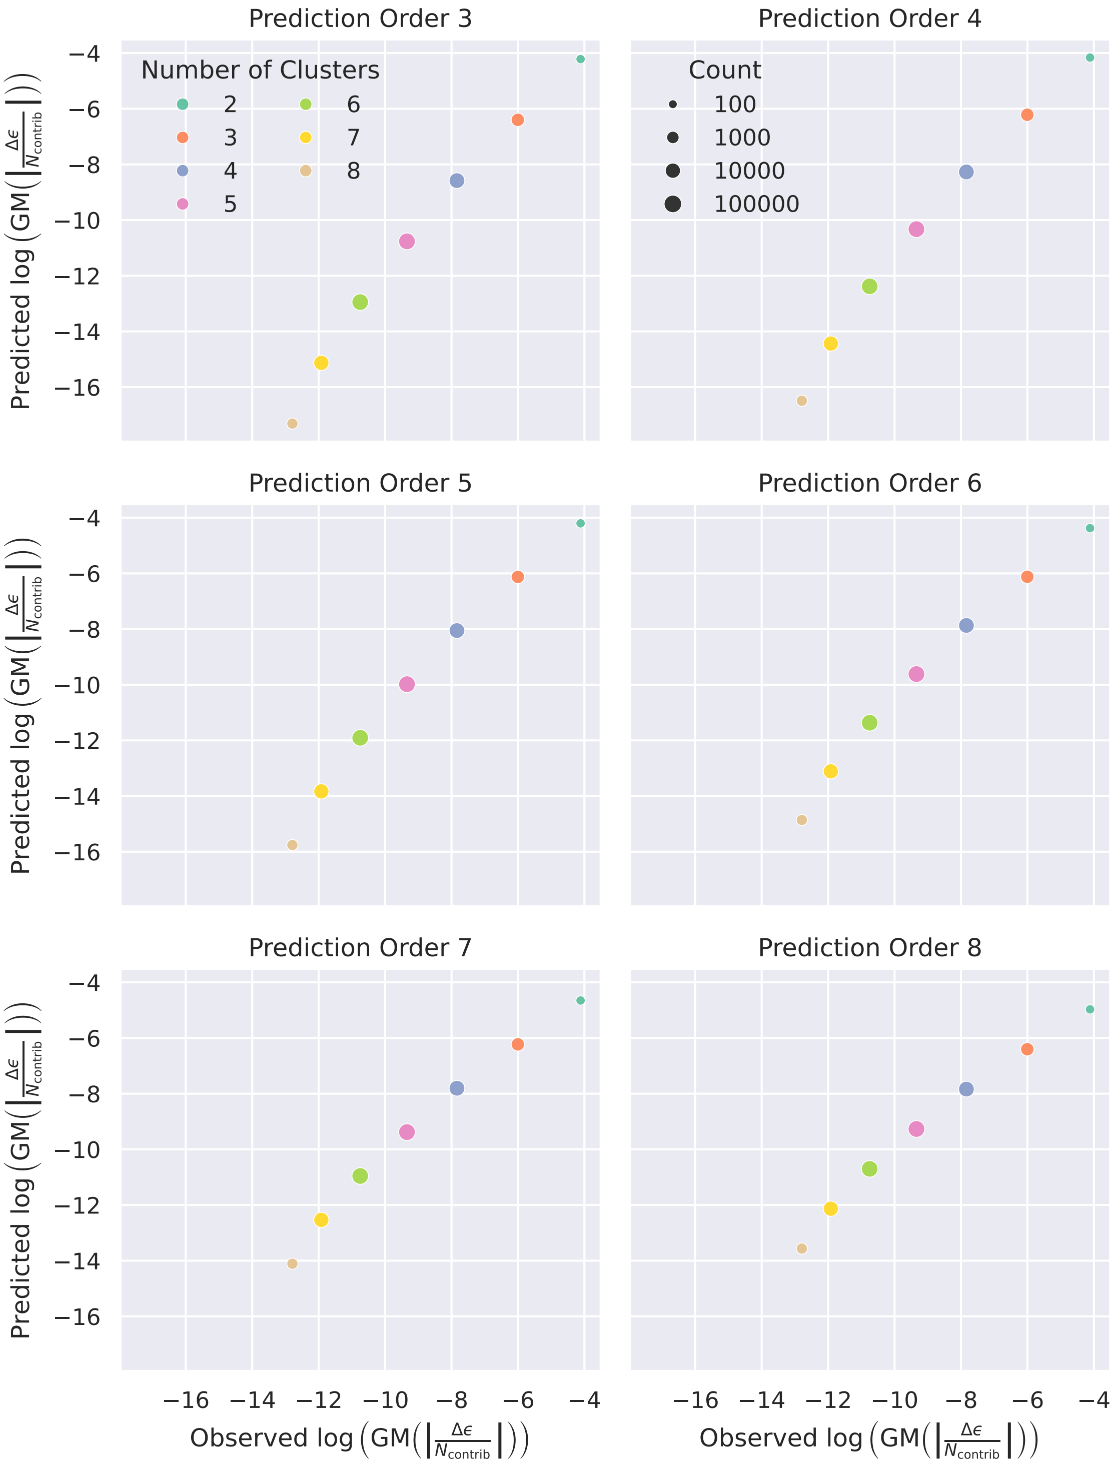


Figure S10: Results for $NH_3$/cc-pVTZ on par with Fig. 3 of the main study.

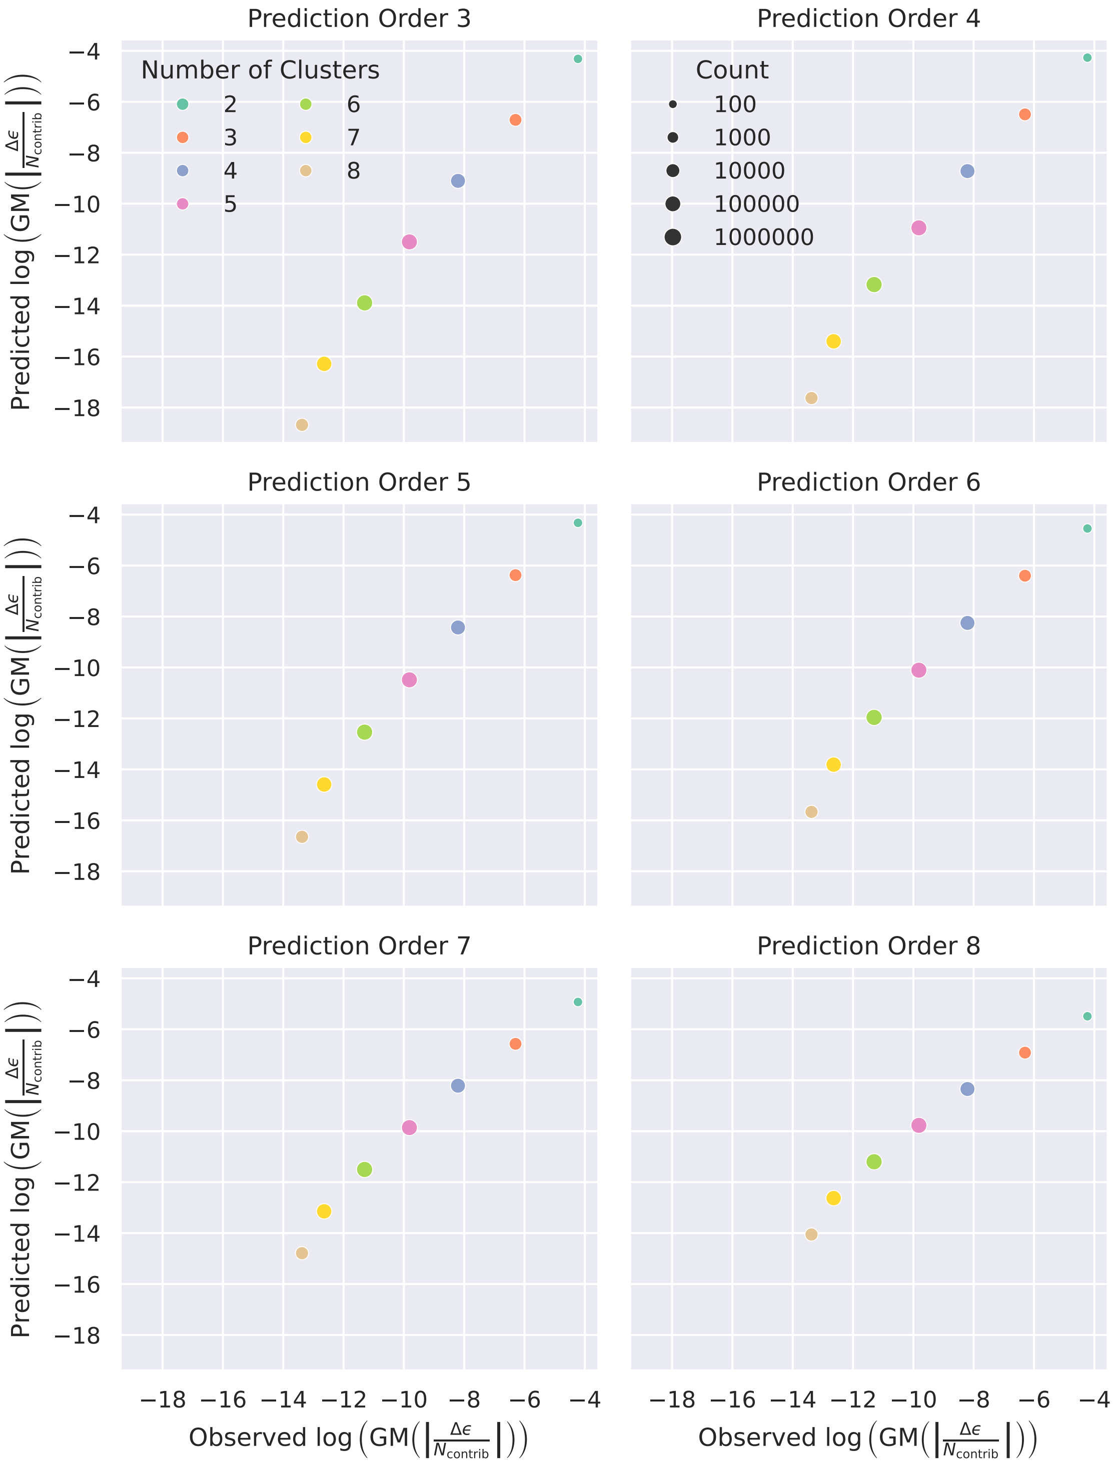


Figure S11: Results for $CH_4$/cc-pVTZ on par with Fig. 3 of the main study.

# 5 Additional Timings

Fig. S12 reports detailed timings in support of Fig. 6 of the main study.

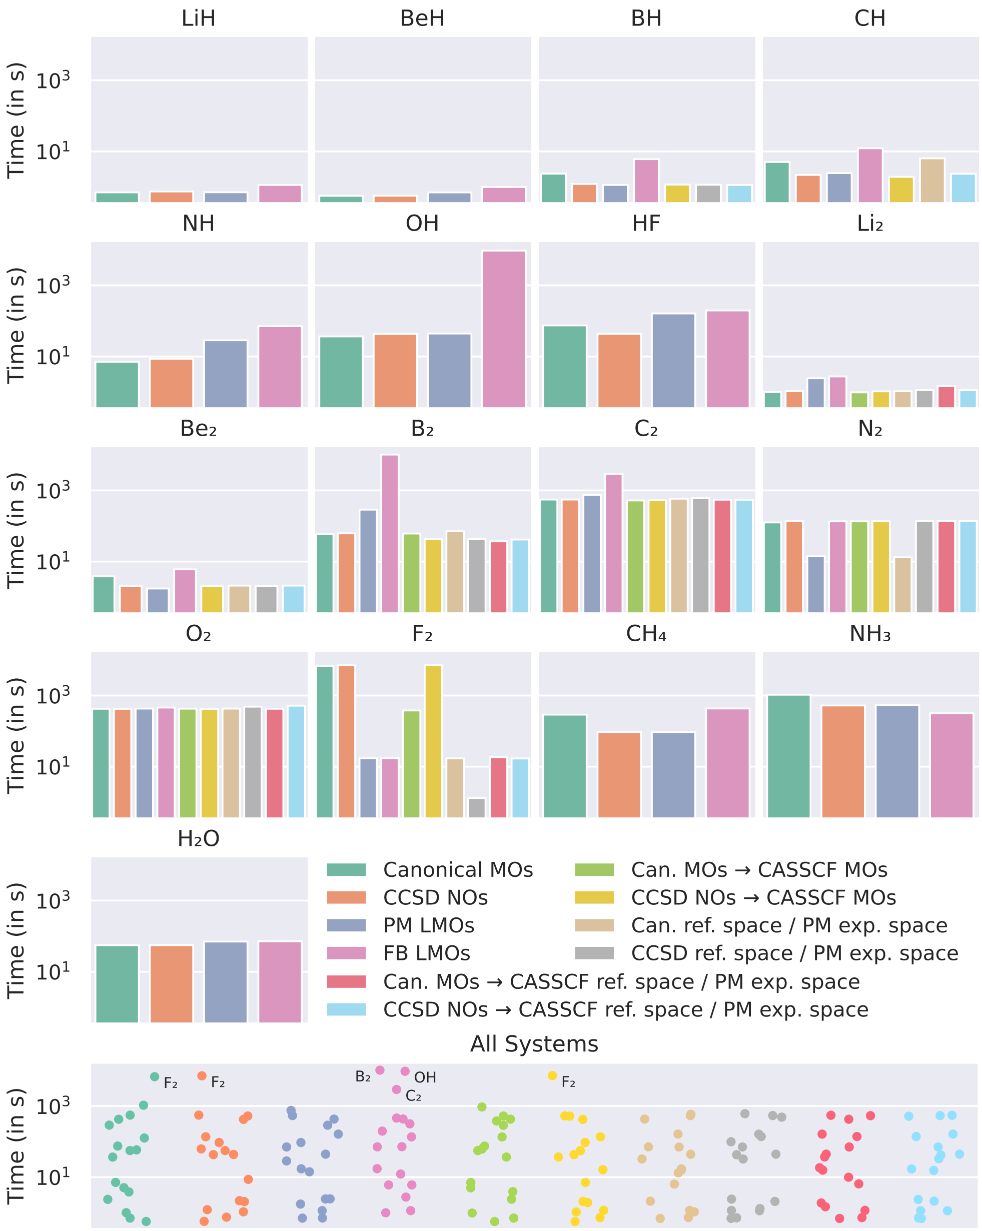


Figure S12: MBE-FCI timings of the `FCI21` set for different MO bases.

For the small systems of the `FCI21` set, the effect of orbital localization is often minor, albeit not insignificant, as is obvious when looking at timings for $N_2$, $F_2$, $CH_4$, $NH_3$, and $H_2O$.

For the vast majority of the systems considered herein, PM LMOs will lead to a lower time-to-solution in comparison to the FB LMOs. One possible explanation could be that the benchmark set includes many systems for which maintaining $\sigma$-$\pi$ separation of the orbitals might be of relevance. For LiH, BeH, NH and HF, all of which require no reference space beyond the open-shell orbitals, the choice of MO basis appears of minor impact. For BH, which only requires a reference space in a basis of CCSD NOs, the explicit inclusion of this reference space appears to accelerate convergence in comparison to the calculation involving canonical orbitals, but not so in comparison to the calculation based on an empty reference space and PM LMOs in the expansion space. For CH, the CASSCF optimization starting from the NOs of the symmetry-broken CCSD solution will lead to a symmetry-broken solution because the symmetry is no longer constrained to $C_{\infty v}$. For this system, MBE-FCI calculations employing this solution appear to converge more rapidly than calculations based on canonical MOs that otherwise describe the correct symmetry state. For the OH system, any benefits from using the large reference space detected in the FB LMO basis obviously fail to materialize, while all other MO bases produce equally fast converging expansions. Calculations on $Li_2$, $Be_2$, $B_2$ and $C_2$ all show no benefits from optimizing reference space orbitals nor localizing expansion space orbitals. In contrast, for $N_2$, PM LMOs again positively affect MBE convergence.

For the systems of the `FCI21` set, optimizing reference space orbitals using CASSCF appears to offer no additional benefit. For such benefits to emerge, systems will likely need be more statically correlated than those studied here. Additionally, it might be necessary to perform the CASSCF optimization after every MBE-FCI restart, which could result in smaller reference spaces by removing correlation from the expansion space before each restart.

# 6 Comparison to DMRG in Canonical Orbitals

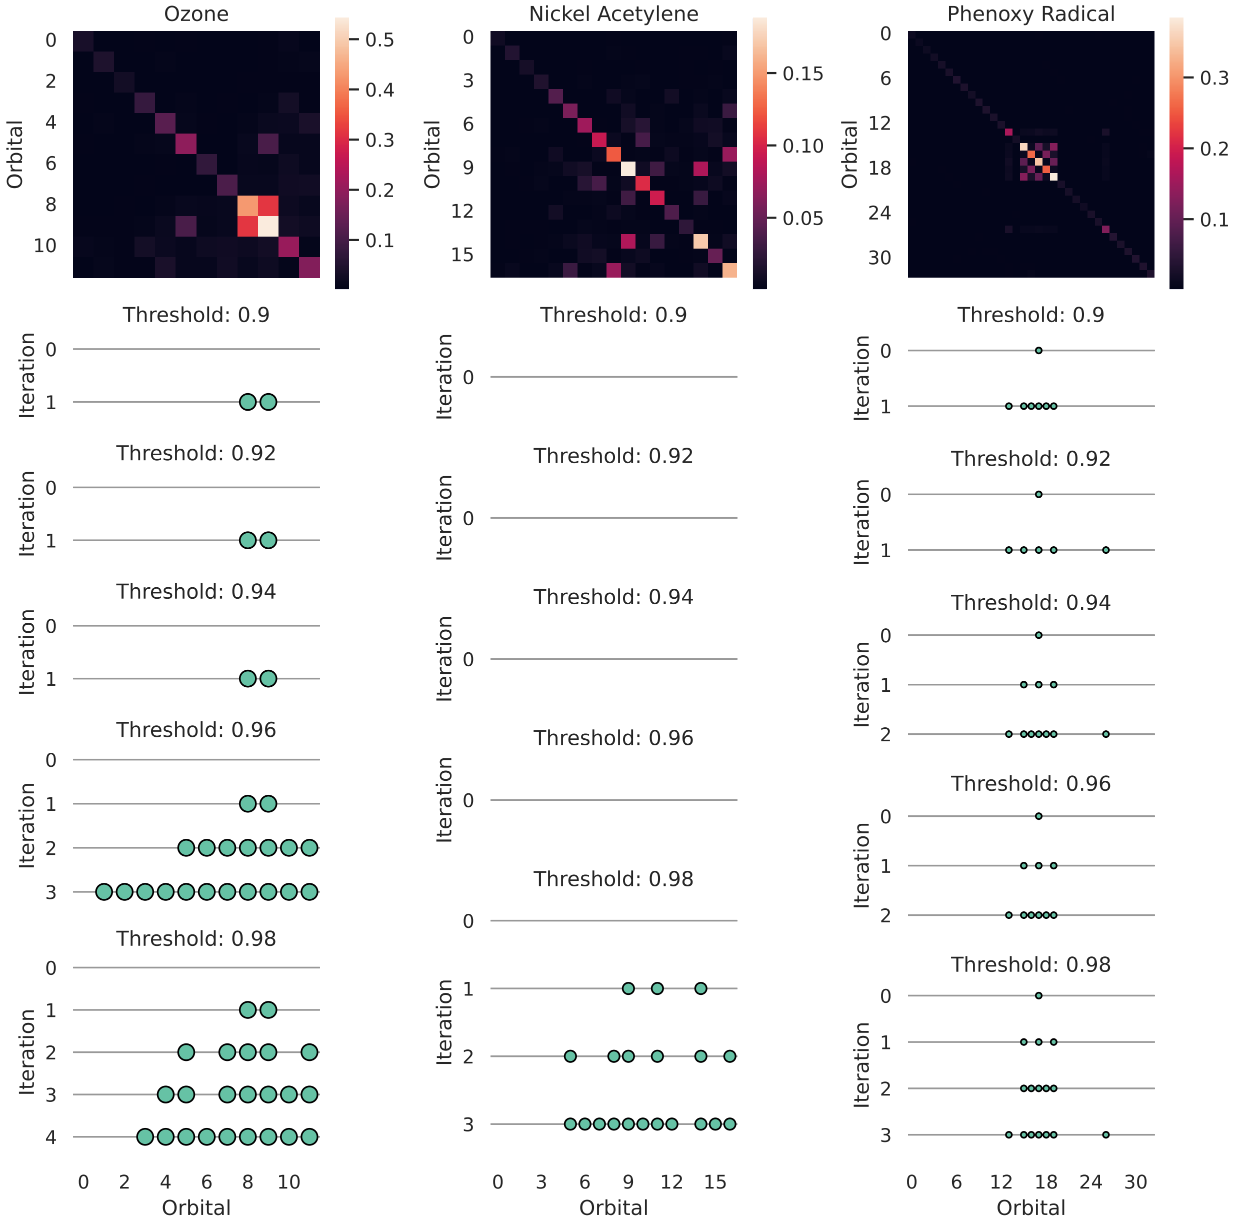


Figure S13: Same results as in Fig. 7 of the main study, but expressed in canonical MOs.

# References


(S1) Fales, B. S.; Hohenstein, E. G.; Levine, B. G. Robust and Efficient Spin Purification for Determinantal Configuration Interaction. J. Chem. Theory Comput. **2017**, 13, 4162.

(S2) Butscher, W.; Kammer, W. Modification of Davidson's Method for the Calculation of Eigenvalues and Eigenvectors of Large Real-Symmetric Matrices: "Root Homing Procedure". J. Comput. Phys. **1976**, 20, 313.

(S3) Ben-Ameur, W. Computing the Initial Temperature of Simulated Annealing. Comput. Optim. Appl. **2004**, 29, 369.

(S4) Rosenblatt, M. Remarks on Some Nonparametric Estimates of a Density Function. Ann. Math. Stat. **1956**, 27, 832.

(S5) Parzen, E. On Estimation of a Probability Density Function and Mode. Ann. Math. Stat. **1962**, 33, 1065.
